# Supplementary material for: GIFT-SW: Gaussian noise Injected Fine-Tuning of Salient Weights for LLMs
Source: arXiv:2408.15300 source file (2024-08-27)
Supplement: Supplementary file 1 [file archive_appendix.tex]

\section{Uniform quantization} \label{appendix:uniform quantization}
While non-uniform quantization may lead to higher compression rates in our work we focus on uniform quantization since quantization is not the main focus of our work. Quantization is a mapping  that converts a range of values into a discrete range of values allowing usage of integer arithmetic and reduced memory consumption. Computations of uniform quantization, de-quantization and estimation of scale parameter $s$ can be performed as below, where parameters $q_{min}$ and $ q_{max}$ depend on a number of bits used for signed quantization as follows: $&q_{min}=-2^{Bit-1}$ and $q_{max}=2^{Bit-1}-1$.

\begin{align}
  z &= -\frac{q_{\text{min}}}{s} \\
  \text{clamp}(x; q_{\text{min}}, q_{\text{max}}) &= \max(q_{\text{min}},\min(x,q_{\text{max}})) \\
\label{eq:quantization}  \mathbf{W}_{\text{int}} &= Q(\mathbf{W}) = \text{clamp}\left(\left\lfloor\frac{\mathbf{W}}{s} + z\right\rfloor; q_{\text{min}}, q_{\text{max}}\right) \\
  s &= \frac{\max(\mathbf{W}) - \min(\mathbf{W})}{q_{\text{max}}} \\
  \mathbf{W} &\approx \hat{\mathbf{W}} = s(x_{\text{int}}-z)
\end{align}


Figure~\ref{fig:step_function} depicts a mapping into integer values with $s=\frac{1}{4}$ and $z=0$. 

For the given bit-width, the parameter $\alpha_{i}$ is found for each row by performing linear grid search over the interval $[0, \max(\mathbf{W}_{[i, frozen]})]$, where $\max(\mathbf{W}_{[i, frozen]})$ is maximum element of the row. The search is conducted to minimize layer-wise quantization error
\hspace{-0.5em}
\begin{equation}
  \label{eq:layerwise_quant_error}
  \mathrm{argmin}_{\tilde{\mathbf{W}}} \Vert \mathbf{W} \mathbf{X} - \tilde{\mathbf{W}} \mathbf{X} \Vert_{2}^{2},
\end{equation}
where $\tilde{\mathbf{W}}$ is the quantized weight obtaining for the quantization step Eq. \ref{eq:quantization}.


\begin{figure}
\centering
\begin{tikzpicture}
\begin{axis}[
    ylabel={$Q(\mathbf{w})$}, % label for x-axis
    xlabel={$\mathbf{w}$}, % label for y-axis
    xtick distance=0.25, % distance between major ticks on the x-axis
    ytick distance=1, % distance between major ticks on the y-axis
    grid=major, % enable grid lines
    ymin=0, ymax=4, % y-axis limits
    xmin=0, xmax=1, % x-axis limits
    axis lines=middle, % put the x and y axis in the middle
    no markers, % don't put markers at points
    samples=100, % number of samples
    domain=0:1, % domain of the function
    ]

    % define the step function
    \addplot+[const plot, thick, blue] coordinates {(0,1) (0.25,2) (0.5,3) (0.75,4) (1,4)};
\addplot+[only text, mark=triangle, mark options={fill=green, draw=green}] coordinates {(0.75,3.2)} node[above, left, blue] { $\Delta$ bit width};
\end{axis}
\end{tikzpicture}
\caption{Uniform quantization step function with real valued one dimensional $\mathbf{w}$ and integer valued $Q(\mathbf{w})$.}
\label{fig:step_function}
\end{figure}


\section{Quantization details} \label{appendix:uniform quantization}
Add technical details on the number of scales etc ...
\textbf{
In our experiments we use MSE to find more optimal $s$ since some weights may contain extreme values. Explain mode and refer to the paper, I think QUIK.
}
\section{Straight Through Estimator} \label{appendix: STE}
STE can be described in two steps:

\begin{itemize}
    \item  Obtain quantized weights $\hat{\theta} \leftarrow Q(\theta)$ from the real-valued parameters $\theta$ with some quantization function $Q$, which is usually is non differentiable.
    \item Compute gradients at quantized weights $\hat{\theta}$ and update real valued weights  $\theta_{t+1} \leftarrow \theta_{t} - \tau \nabla f(\hat{\theta_{t}})$
\end{itemize}
STE makes a particular choice of a quantization function to obtain the discrete weights from the real-valued weights. This approximation can be justified in some settings \citep{lin2017towards} but in general the reasons behind its effectiveness are unknown.

\section{Detailed Benchmark Results} \label{appendix:bench_results}

\input{latex/full_fp_tables}
\input{latex/full_quant}
